# Supplementary material for: Large-Scale Low-Rank Matrix Learning with Nonconvex Regularizers
Source: arXiv:1708.00146 source file (2018-07-23)
Supplement: Supplementary file 1 [file appendix.pdf]

# Appendix A
# Proofs

## A.1 Proposition 3.1

For simplicity of notations, we write $\sigma_i(\mathbf{Z})$ as $\sigma_i$. First, we introduce the definition of super-gradient for a concave function and two lemmas.

**Definition 2** ( [47]). *For a concave function $f$, its super-gradient is given by $g \in \hat{\partial} f \equiv \partial(-f)$.*

**Lemma A.1** ( [47]). *(i) $\inf_{g \in \hat{\partial}\hat{r}(y)} g \geq 0$; (ii) Assume that $y_j \geq y_i \geq 0$. Then, $\sup_{g_j \in \hat{\partial}\hat{r}(y_j)} g_j \leq \inf_{g_i \in \hat{\partial}\hat{r}(y_i)} g_i$.*

**Lemma A.2.** *(i) $y_i^* - \max(\sigma_i - \mu g_i, 0) = 0$, where $g_i \in \hat{\partial}\hat{r}(y_i^*)$; (ii) if $y_i^* > 0$, then $y_i^*$ increases with $\sigma_i$.*

*Proof.* (Part (i)): Let $g_i \in \hat{\partial}\hat{r}(y_i^*)$. From the first-order optimality condition of (4), consider the two possibilities:

(a) $\underline{\sigma_i + \mu g_i \leq 0}$: In other words, the optimal solution is achieved at the boundary, and $y_i^* = 0$.

(b) $\underline{\sigma_i + \mu g_i > 0}$: We have $0 = y_i^* - \sigma_i + \mu g_i$, and $y_i^* > 0$.

Combining these two cases, the relationship between $y_i^*$ and $\sigma_i$ can be expressed as

$$y_i^* = \max(\sigma_i - \mu g_i, 0). \tag{13}$$

(Part (ii)): Assume that $y_i^* > 0$. Then, (13) becomes

$$y_i^* = \sigma_i - \mu g_i. \tag{14}$$

Let $\sigma_i$ becomes larger as $\sigma_j$. according to (14), we have two possibilities for its corresponding $y_j^*$, i.e.,

- $\underline{y_j^* > y_i^*}$: Then, $\sup_{g_j \in \hat{\partial}\hat{r}(y_j^*)} g_j \leq \inf_{g_i \in \hat{\partial}\hat{r}(y_i^*)} g_i$ from Lemma A.1. Together with the fact that $\sigma_j > \sigma_i$, there exists a $y_j^*$ which is not smaller than $y_i^*$ to make (13) hold.
- $\underline{y_j^* \leq y_i^*}$: Then, $\inf_{g_j \in \hat{\partial}\hat{r}(y_j^*)} g_j \geq \sup_{g_i \in \hat{\partial}\hat{r}(y_i^*)} g_i$ from Lemma A.1. However, such a solution may not exist (e.g., when $\hat{r}(\alpha) = \alpha$).

Thus, while there can be multiple solutions to ensure (14), the first case must exist. We take the largest solution of all possible candidates. Thus, if $\sigma_i$ gets larger, $y_i^*$ also becomes larger.

□

*Proof of Proposition 3.1.* From Lemma A.2, we have

$$0 = y_i^* - \max(\sigma_i - \mu g_i, 0).$$

We can see that $y^* = 0$ once $\sigma_i - \mu g_i \leq 0$. However, if $\sigma_i$ becomes smaller, $\sigma_i - \mu g_i$ will reach 0 before $\sigma_i$ reaches zero. This comes from two facts. First, $y_i^*$ becomes smaller as $\sigma_i$ gets smaller (Lemma A.2), but $\inf_{g_i \in \hat{\partial}\hat{r}(y_i^*)} g_i$ will not become smaller (Lemma A.1). Second, we have $\lim_{y \to 0^+} \inf_{g \in \hat{\partial}\hat{r}(y)} g > 0$. An illustration of the relationships among $\sigma_i$, $y_i^*$ and $g_i$ is shown in the following Figure 16. Thus, there exists $\gamma > 0$ such that once $\sigma_i \leq \gamma$, $\sigma_i - \mu g_i \leq 0$, and $y_i^*$ becomes 0.

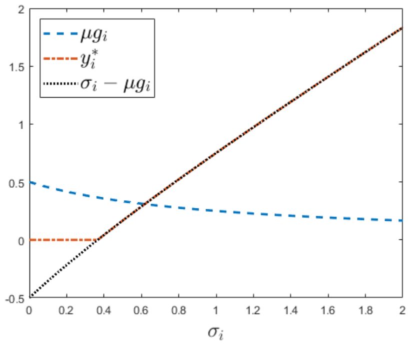


Fig. 16. Illustration of Proposition 3.1.

## A.2 Corollary 3.2

In this section, we show how to derive the threshold $\gamma$ for the capped-$\ell_1$ penalty. Derivations for the other penalties can be obtained similarly.

### A.2.1 Capped-$\ell_1$ Penalty

*Proof.* Note that problem (4) considers each singular value separately. For simplicity of notations, let $\sigma_i$ denote $\sigma_i(\mathbf{Z})$. For the $i$th singular value, let

$$h(y_i) \equiv \frac{1}{2}(y_i - \sigma_i)^2 + \mu \min(y_i, \theta).$$

Thus,

$$\operatorname{Arg}\min_{y_i \geq 0} h(y_i) = \begin{cases} \operatorname{Arg}\min_{0 \leq y_i \leq \theta} h_1(y_i) \\ \operatorname{Arg}\min_{y_i > \theta} h_2(y_i) \end{cases},$$

where

$$h_1(p_i) = \frac{1}{2}(p_i - \sigma_i)^2 + \mu p_i,$$
$$h_2(q_i) = \frac{1}{2}(q_i - \sigma_i)^2 + \mu\theta.$$

Note that $h_1$ is quadratic. There are only three possibilities for $p_i^* = \operatorname{Arg}\min_{0 \leq p_i \leq \theta} h_1(p_i)$, i.e.,

$$\min_{0 \leq p_i \leq \theta} h_1(p_i) = \begin{cases} \frac{1}{2}\sigma_i^2 & \text{if } p_i^* = 0 \\ \mu\sigma_i - \frac{1}{2}\mu^2 & \text{if } p_i^* = \sigma_i - \mu \\ \frac{1}{2}(\theta - \sigma_i)^2 + \mu\sigma_i & \text{if } p_i^* = \theta \end{cases},$$

and

$$p_i^* = \begin{cases} 0 & \text{if } 0 \leq \sigma_i \leq \mu \\ \sigma_i - \mu & \text{if } \mu < \sigma_i \leq \mu + \theta \\ \theta & \text{otherwise} \end{cases}. \tag{15}$$

Let $q_i^* = \operatorname{Arg}\min_{q_i > \theta} h_2(q_i)$. As $h_2$ is also quadratic and $q_i^*$ cannot be $\theta$, we have

$$q_i^* = \begin{cases} \text{no solution} & \text{if } 0 \leq \sigma_i \leq \theta \\ \sigma_i & \text{otherwise} \end{cases}. \tag{16}$$

Note that when $\sigma_i \in [0, \theta]$, there is no solution to $q_i^*$, as $q_i^*$ can arbitrarily close to $\theta$. Since $h_1(\theta) = h_2(\theta)$, the possibility for $\theta = \operatorname{Arg}\min_{y_i \geq 0} h(y_i)$ is covered by $\operatorname{Arg}\min_{0 \leq p_i \leq \theta} h_1$. Thus, (15) and (16) have covered all possibilities of $y_i^*$. Using them, we have

1) If $\theta \leq \mu$, then

$$\min_{y_i \geq 0} h = \begin{cases} h_1(0) & 0 \leq \sigma_i \leq \theta \\ \min(h_1(0), h_2(\sigma_i)) & \theta < \sigma_i \leq \mu \\ \min(h_1(\sigma_i - \mu), h_2(\sigma_i)) & \mu < \sigma_i \leq \mu + \theta \\ \min(h_1(\theta), h_2(\sigma_i)) & \sigma_i > \mu + \theta \end{cases}.$$

In order to get $y_i^* = 0$, we need

$$\min\left(h_1(0), h_2(\sigma_i)\right) = h_1(0),$$

which leads to

$$\sigma_i \leq \sqrt{2\mu\theta}.$$

Thus, if $0 \leq \sigma_i \leq \min\left(\sqrt{2\mu\theta}, \mu\right)$, then $y_i^* = 0$.

2) If $\theta > \mu$, then

$$\min_{y_i \geq 0} h = \begin{cases} h_1(0) & 0 \leq \sigma_i \leq \mu \\ h_1(\sigma_i - \mu) & \mu < \sigma_i \leq \theta \\ \min\left(h_1(\sigma_i - \mu), h_2(\sigma_i)\right) & \theta < \sigma_i \leq \mu + \theta \\ \min\left(h_1(\theta), h_2(\sigma_i)\right) & \sigma_i > \mu + \theta \end{cases}.$$

Thus, if $0 \leq \sigma_i \leq \mu$, then we have $y_i^* = 0$.

Finally, combining the above two cases, we can conclude that once $\sigma_i \leq \min(\sqrt{2\theta\mu}, \mu)$, then $y_i^* = 0$. Thus, $\gamma = \min(\sqrt{2\theta\mu}, \mu)$. □

### A.3 Proposition 3.3

*Proof.* First, we introduce the following theorem.

**Theorem A.3** (Separation theorem [48]). *Let $\mathbf{X}_{gd} \in \mathbb{R}^{m\times n}$ and $\mathbf{B} \in \mathbb{R}^{m\times r}$ with $\mathbf{B}^\top\mathbf{B} = \mathbf{I}$. Then*

$$\sigma_i\left(\mathbf{B}^\top\mathbf{X}_{gd}\right) \leq \sigma_i(\mathbf{X}_{gd}), \text{ for } i = 1, \dots, \min(r, n).$$

Let the SVD of $\mathbf{Z}$ be $\mathbf{U}\mathbf{\Sigma}\mathbf{V}^\top$. $\mathbf{Z}$ can then be rewritten as

$$\mathbf{Z} = [\mathbf{U}_{\hat{k}}; \mathbf{U}_\perp]\begin{bmatrix}\mathbf{\Sigma}_{\hat{k}} & \\ & \mathbf{\Sigma}_\perp\end{bmatrix}[\mathbf{V}_{\hat{k}}; \mathbf{V}_\perp]^\top, \quad (17)$$

where $\mathbf{U}_{\hat{k}}$ contains the $\hat{k}$ leading columns of $\mathbf{U}$, and $\mathbf{U}_\perp$ the remaining columns. Similarly, $\mathbf{\Sigma}_{\hat{k}}$ (resp. $\mathbf{V}_{\hat{k}}$) contains the $\hat{k}$ leading eigenvalues (resp. columns) of $\mathbf{\Sigma}$ (resp. $\mathbf{V}$). Let

$$\tilde{\mathbf{u}}_i = \mathbf{Q}^\top\mathbf{u}_i \quad \text{and} \quad \tilde{\mathbf{v}}_i = \mathbf{v}_i, \quad (18)$$

where $\mathbf{u}_i$ (resp. $\mathbf{v}_i$) is the $i$th column of $\mathbf{U}$ (resp. $\mathbf{V}$). Then, for $i = 1, \dots, \hat{k}$, we have

$$\begin{aligned}\tilde{\mathbf{u}}_i^\top\left(\mathbf{Q}^\top\mathbf{Z}\right)\tilde{\mathbf{v}}_i &= \mathbf{u}_i^\top\left(\mathbf{Q}\mathbf{Q}^\top\right)\mathbf{Z}\mathbf{v}_i \\ &= \mathbf{u}_i^\top\mathbf{Z}\mathbf{v}_i \quad (19)\\ &= \sigma_i(\mathbf{Z}), \quad (20)\end{aligned}$$

where (19) is due to $\text{span}(\mathbf{U}_{\hat{k}}) \subseteq \text{span}(\mathbf{Q})$. Hence,

$$\sigma_i\left(\mathbf{Q}^\top\mathbf{Z}\right) = \sigma_i(\mathbf{Z}), \text{ for } i = 1, \dots, \hat{k}. \quad (21)$$

From Theorem A.3, by substituting $\mathbf{Q} = \mathbf{B}$ and $\mathbf{X}_{\text{gd}} = \mathbf{Z}$, we have $\sigma_i(\mathbf{Q}^\top\mathbf{Z}) \leq \sigma_i(\mathbf{Z})$. Combining with (20), we obtain that the rank-$\hat{k}$ SVD of $\mathbf{Q}^\top\mathbf{Z}$ is $(\mathbf{Q}^\top\mathbf{U}_{\hat{k}})\mathbf{\Sigma}_{\hat{k}}\mathbf{V}_{\hat{k}}^\top$, with the corresponding left and right singular vectors contained in $\mathbf{Q}^\top\mathbf{U}_{\hat{k}}$ and $\mathbf{V}_{\hat{k}}$, respectively.

Again, by Theorem A.3, we have

$$\sigma_{\hat{k}+1}\left(\mathbf{Q}^\top\mathbf{Z}\right) \leq \sigma_{\hat{k}+1}(\mathbf{Z}) \leq \gamma.$$

Besides, using (17),

$$\sigma_i\left(\mathbf{Q}^\top\mathbf{Z}\right) = \max_{\tilde{\mathbf{u}}_i, \tilde{\mathbf{v}}_i} \tilde{\mathbf{u}}_i^\top\left(\mathbf{Q}^\top\mathbf{U}_{\hat{k}}\mathbf{\Sigma}_{\hat{k}}\mathbf{V}_{\hat{k}}^\top + \mathbf{Q}^\top\mathbf{U}_\perp\mathbf{\Sigma}_\perp\mathbf{V}_\perp^\top\right)\tilde{\mathbf{v}}_i.$$

The first $\hat{k}$ singular values are from the term $\mathbf{Q}^\top\mathbf{U}_{\hat{k}}\mathbf{\Sigma}_{\hat{k}}\mathbf{V}_{\hat{k}}$. Hence,

$$\sigma_{\hat{k}+1}\left(\mathbf{Q}^\top\mathbf{Z}\right) = \max_{\tilde{\mathbf{u}}, \tilde{\mathbf{v}}} \tilde{\mathbf{u}}^\top\left(\mathbf{Q}^\top\mathbf{U}_\perp\mathbf{\Sigma}_\perp\mathbf{V}_\perp^\top\right)\tilde{\mathbf{v}} \leq \gamma. \quad (22)$$

Then,

$$\begin{aligned}&\text{prox}_{\mu r}(\mathbf{Q}^\top\mathbf{Z}) \\ &= \text{prox}_{\mu r}(\mathbf{Q}^\top\mathbf{U}_{\hat{k}}\mathbf{\Sigma}_{\hat{k}}\mathbf{V}_{\hat{k}}^\top + \mathbf{Q}^\top\mathbf{U}_\perp\mathbf{\Sigma}_\perp\mathbf{V}_\perp^\top) \\ &= \text{prox}_{\mu r}(\mathbf{Q}^\top\mathbf{U}_{\hat{k}}\mathbf{\Sigma}_{\hat{k}}\mathbf{V}_{\hat{k}}^\top) + \text{prox}_{\mu r}(\mathbf{Q}^\top\mathbf{U}_\perp\mathbf{\Sigma}_\perp\mathbf{V}_\perp^\top) \quad (23)\\ &= \text{prox}_{\mu r}(\mathbf{Q}^\top\mathbf{U}_{\hat{k}}\mathbf{\Sigma}_{\hat{k}}\mathbf{V}_{\hat{k}}^\top). \quad (24)\end{aligned}$$

where (23) follows from that $\mathbf{Q}^\top\mathbf{U}_{\hat{k}}$ (resp. $\mathbf{V}_{\hat{k}}$) is orthogonal to $\mathbf{Q}\mathbf{U}_\perp$ (resp. $\mathbf{V}_\perp$). (22) shows that there are only $\hat{k}$ singular values in $\mathbf{Q}^\top\mathbf{Z}$ larger than $\gamma$. Thus, $\text{prox}_{\mu r}(\mathbf{Q}^\top\mathbf{U}_\perp\mathbf{\Sigma}_\perp\mathbf{V}_\perp^\top) = 0$ and we get (24). Finally,

$$\begin{aligned}\mathbf{Q}\text{prox}_{\mu r}(\mathbf{Q}^\top\mathbf{Z}) &= \mathbf{Q}\left(\mathbf{Q}^\top\mathbf{U}_{\hat{k}}\text{prox}_{\mu r}(\mathbf{\Sigma}_{\hat{k}})\mathbf{V}_{\hat{k}}^\top\right) \\ &= \mathbf{U}_{\hat{k}}\text{prox}_{\mu r}(\mathbf{\Sigma}_{\hat{k}})\mathbf{V}_{\hat{k}}^\top \quad (25)\\ &= \text{prox}_{\mu r}(\mathbf{Z}), \quad (26)\end{aligned}$$

where (25) comes from $\text{span}(\mathbf{U}_{\hat{k}}) \subseteq \text{span}(\mathbf{Q})$; (26) comes from that rank-$\hat{k}$ SVD of $\mathbf{Z}$ is $\mathbf{U}_{\hat{k}}\mathbf{\Sigma}_{\hat{k}}\mathbf{V}_{\hat{k}}^\top$ and $\mathbf{Z}$ only has $\hat{k}$ singular values larger than $\gamma$. □

### A.4 Proposition 3.5

*Proof.* First, we introduce the following Lemmas.

**Lemma A.4** ( [27]). *In Algorithm 1, let the SVD of $\mathbf{Z}$ be $\bar{\mathbf{U}}\bar{\mathbf{\Sigma}}\bar{\mathbf{V}}^\top$, and $\bar{\mathbf{U}}_k$ contain the first $k$ columns of $\bar{\mathbf{U}}$. We have*

$$\|\mathbf{Q}_j\mathbf{Q}_j^\top - \bar{\mathbf{U}}_k\bar{\mathbf{U}}_k^\top\|_F \leq \alpha^{j-1}\|\mathbf{C}\mathbf{C}^\top - \bar{\mathbf{U}}_k\bar{\mathbf{U}}_k^\top\|_F,$$

*where $\alpha = \sigma_{k+1}(\mathbf{Z})/\sigma_k(\mathbf{Z}) \in (0, 1)$ and $\mathbf{C} = \text{QR}(\mathbf{Z}\mathbf{R})$.*

**Lemma A.5.** *In Algorithm 3, let the rank-$k$ SVD of $\mathbf{X}_{gd}$ be $\mathbf{U}_k\mathbf{\Sigma}_k\mathbf{V}_k^\top$, and*

$$\mathbf{B}_p = \text{QR}(\mathbf{X}_{gd}\tilde{\mathbf{V}}_p). \quad (27)$$

*Then, $\|\mathbf{B}_p\mathbf{B}_p^\top - \mathbf{U}_k\mathbf{U}_k^\top\|_F \leq \eta^p\|\mathbf{B}_0\mathbf{B}_0^\top - \mathbf{U}_k\mathbf{U}_k^\top\|_F$, where $\eta \in (0, 1)$ is a constant.*

*Proof.* At the $p$th iteration of Algorithm 3, inside Algorithm 1 (step 3), since $\mathbf{Z} = \mathbf{X}_{\text{gd}}$ and $\mathbf{R} = \tilde{\mathbf{V}}_{p-1}$, we have

$$\mathbf{Q}_1 = \text{QR}(\mathbf{X}_{\text{gd}}\tilde{\mathbf{V}}_{p-1}) = \mathbf{B}_{p-1}. \quad (28)$$

Then, for $\tilde{\mathbf{V}}_p$, inside Algorithm 2 (step 2), we have

$$\text{span}(\tilde{\mathbf{V}}_p) = \text{span}(\mathbf{X}_{\text{gd}}^\top\mathbf{Q}).$$

Thus,

$$\begin{aligned}\text{span}(\mathbf{X}_{\text{gd}}\tilde{\mathbf{V}}_p) &= \text{span}(\mathbf{X}_{\text{gd}}(\mathbf{X}_{\text{gd}}^\top\mathbf{Q})) \\ &= \text{span}(\mathbf{X}_{\text{gd}}(\mathbf{X}_{\text{gd}}^\top\mathbf{Q}_J)) \quad (29)\\ &= \text{span}(\mathbf{Y}_{J+1}), \quad (30)\end{aligned}$$

where (29) comes from the fact that $\mathbf{Q}$ is returned after $J$ iterations of Algorithm 1; and (30) from the definition of $\mathbf{Y}_{j+1}$ at step 4 in Algorithm 1. Thus,

$$\begin{aligned}\mathbf{Q}_{J+1} &= \text{QR}(\mathbf{Y}_{J+1}) \\ &= \text{QR}(\mathbf{X}_{\text{gd}}\tilde{\mathbf{V}}_p) = \mathbf{B}_p. \quad (31)\end{aligned}$$

Note that $\mathbf{C} = \mathbf{Q}_1$ in Lemma A.4. Together with (28) and (31), we have

$$\begin{aligned}\|\mathbf{B}_p\mathbf{B}_p^\top - \mathbf{U}_k\mathbf{U}_k^\top\|_F &= \|\mathbf{Q}_{J+1}\mathbf{Q}_{J+1}^\top - \mathbf{U}_k\mathbf{U}_k^\top\|_F \\ &\le \alpha^J\|\mathbf{Q}_1\mathbf{Q}_1^\top - \mathbf{U}_k\mathbf{U}_k^\top\|_F \\ &= \eta\|\mathbf{B}_{p-1}\mathbf{B}_{p-1}^\top - \mathbf{U}_k\mathbf{U}_k^\top\|_F,\end{aligned}$$

where $\eta = \alpha^J \in (0,1)$. Thus,

$$\|\mathbf{B}_p\mathbf{B}_p^\top - \mathbf{U}_k\mathbf{U}_k^\top\|_F \le \eta^p\|\mathbf{B}_0\mathbf{B}_0^\top - \mathbf{U}_k\mathbf{U}_k^\top\|_F.$$

□

(Proof of Proposition 3.5) For $\mathbf{B}_p$ in (27), we have $\lim_{p\to\infty}\mathbf{B}_p = \mathbf{U}_k$ from Proposition A.5 where $\mathbf{U}_k$ comes from rank-$k$ SVD of $\mathbf{X}_{\text{gd}}$. As $k \ge \hat{k}_{\mathbf{X}_{\text{gd}}}$, $\text{span}(\mathbf{U}_{\hat{k}_{\mathbf{X}_{\text{gd}}}}) \subseteq \text{span}(\mathbf{U}_k)$. Then, from Proposition 3.3, we have

$$\mathbf{U}_k\text{prox}_{\frac{\lambda}{\tau}r}(\mathbf{U}_k^\top\mathbf{X}_{\text{gd}}) = \text{prox}_{\frac{\lambda}{\tau}r}(\mathbf{X}_{\text{gd}}).$$

Thus, $\lim_{p\to\infty}\tilde{\mathbf{X}}_p = \text{prox}_{\frac{\lambda}{\tau}r}(\mathbf{X}_{\text{gd}})$. □

### A.5 Proposition 3.6

*Proof.* First, we introduce Lemma A.6.

**Lemma A.6** ( [49]). *Let $\phi(\mathbf{X}) = \sum_{i=1}^m f(\sigma_i(\mathbf{X}))$. If $f$ is convex, $\phi$ is also convex on $\mathbf{X}$.*

For $\hat{r}$ in Assumption A3, it can be rewritten as $\hat{r}(\alpha) = \hat{r}_1(\alpha) - \hat{r}_2(\alpha)$, where $\hat{r}_1(\alpha) = \kappa\alpha$ (for some constant $\kappa$) and $\hat{r}_2(\alpha) = \kappa\alpha - \hat{r}(\alpha)$. Obviously, both $\hat{r}_1$ and $\hat{r}_2$ are convex. Define

$$\breve{r}(\mathbf{X}) = \sum_{i=1}^m \hat{r}_1(\sigma_i(\mathbf{X})), \text{ and } \tilde{r}(\mathbf{X}) = \sum_{i=1}^m \hat{r}_2(\sigma_i(\mathbf{X})).$$

From Lemma A.6, both $\breve{r}$ and $\tilde{r}$ are convex. Thus, $r$ can also be written as a difference of convex functions: $r(\mathbf{X}) = \breve{r}(\mathbf{X}) - \tilde{r}(\mathbf{X})$. □

### A.6 Proposition 3.7

*Proof.* From step 5 of Algorithm 4 (which ensures (5)), we have

$$F(\mathbf{X}_{t+1}) \le F(\mathbf{X}_t) - c_1\|\mathbf{X}_{t+1} - \mathbf{X}_t\|_F^2.$$

Summing this from $t = 1$ to $T$, we have

$$\begin{aligned} c_1\sum_{t=1}^T\|\mathbf{X}_{t+1} - \mathbf{X}_t\|_F^2 &\le F(\mathbf{X}_1) - F(\mathbf{X}_{T+1}) \\ &\le F(\mathbf{X}_1) - \inf F. \end{aligned} \tag{32}$$

As $F$ is bounded from below (Assumption A2),

$$a_1 \equiv F(\mathbf{X}_1) - \inf F$$

is a positive constant. Let $T \to \infty$, we have

$$\sum_{t=1}^\infty \|\mathbf{X}_{t+1} - \mathbf{X}_t\|_F^2 \le \frac{a_1}{c_1}. \tag{33}$$

From Assumption A2, we also have $\lim_{\|\mathbf{X}\|_F\to\infty} f(\mathbf{X}) \to \infty$. which implies that $\max_{t=1,\dots,\infty}\|\mathbf{X}_t\|_F < \infty$. Together with (33), $\{\mathbf{X}_t\}$ is a bounded sequence with at least one limit point [47]. □

### A.7 Corollary 3.8

*Proof.* Combining (32) and (33), we have

$$\begin{aligned}\min_{t=1,\dots,T}\|\mathbf{X}_{t+1} - \mathbf{X}_t\|_F^2 &\le \frac{1}{T}\sum_{t=1}^T\|\mathbf{X}_{t+1} - \mathbf{X}_t\|_F^2 \\ &\le \frac{1}{T}\sum_{t=1}^\infty\|\mathbf{X}_{t+1} - \mathbf{X}_t\|_F^2 \\ &\le \frac{F(\mathbf{X}_1) - \inf F}{c_1 T}.\end{aligned}$$

□

### A.8 Theorem 3.9

**Lemma A.7.** InexactPS $(\mathbf{X}, \mathbf{R})$, *i.e., Algorithm 3, is a continuous function on its input $\mathbf{X}$ and $\mathbf{R}$.*

*Proof.* Note that the operations inside Algorithm 3 on $\mathbf{X}$ and $\mathbf{R}$ are matrix addition, multiplication, taking gradient of $f$ on $\mathbf{X}$, and QR and SVD. Since (i) matrix addition and multiplication are linear operators; (ii) $f$ is a smooth function; and (iii) QR$(\cdot)$ and SVD$(\cdot)$ are smooth operators on the input matrix [50]. Thus, Algorithm 3 is a continuous function of its input matrices. □

**Lemma A.8** ( [24], [29]). *If $\mathbf{X} = \text{prox}_{\frac{\lambda}{\tau}r}(\mathbf{X} - \frac{1}{\tau}\nabla f(\mathbf{X}))$, then $\mathbf{X}$ is a critical point of* (1).

*Proof.* (Theorem 3.9) As $\{\mathbf{X}_{t_j}\}$ is a subsequence of $\{\mathbf{X}_t\}$ with limit point $\mathbf{X}_*$,

$$\lim_{t_j\to\infty}\mathbf{X}_{t_j+1} = \lim_{t_j\to\infty}\text{InexactPS}\left(\mathbf{X}_{t_j}, \mathbf{R}_{t_j}\right), \tag{34}$$

$$= \text{InexactPS}\left(\lim_{t_j\to\infty}\mathbf{X}_{t_j}, \lim_{t_j\to\infty}\mathbf{R}_{t_j}\right), \tag{35}$$

where (34) is due to continuity of InexactPS$(\cdot,\cdot)$ (Lemma A.7). Then, from (33), we have $\lim_{t\to\infty}\|\mathbf{X}_{t+1} - \mathbf{X}_t\|_F^2 = 0$. which implies

$$\lim_{t_j\to\infty}\mathbf{X}_{t_j+1} = \lim_{t_j\to\infty}\mathbf{X}_{t_j} = \mathbf{X}_*, \tag{36}$$

for $\{\mathbf{X}_{t_j}\}$. Combining (35) and (36), we have

$$\begin{aligned}\lim_{t_j\to\infty}\mathbf{X}_* &= \text{InexactPS}\left(\lim_{t_j\to\infty}\mathbf{X}_{t_j}, \lim_{t_j\to\infty}\mathbf{R}_{t_j}\right), \\ &= \text{InexactPS}\left(\mathbf{X}_*, \lim_{t_j\to\infty}\mathbf{R}_{t_j}\right).\end{aligned}$$

Thus, $\mathbf{X}_* = \text{prox}_{\frac{\lambda}{\tau}r}(\mathbf{X}_* - \frac{1}{\tau}\nabla f(\mathbf{X}_*))$ holds by the assumption. From Lemma A.8, $\mathbf{X}_*$ is a critical point of (1). □

### A.9 Proposition 3.10

*Proof.* Consider the two cases:

1) Step 8 in Algorithm 5 is performed: Then,

$$F(\mathbf{X}_{t+1}) \le F(\mathbf{X}_t) - \frac{\delta}{2}\|\mathbf{X}_{t+1} - \mathbf{Y}_t\|_F^2. \tag{37}$$

2) Step 10 is performed: Then,

$$F(\mathbf{X}_{t+1}) \le F(\mathbf{X}_t) - c_1\|\mathbf{X}_{t+1} - \mathbf{X}_t\|_F^2. \tag{38}$$

Partition the iterations $\{1, \ldots, T\}$ into two sets $\Omega_T^1$ and $\Omega_T^2$, such that $t \in \Omega_T^1$ if step 8 is performed, and $t \in \Omega_T^2$ if step 10 is performed. Sum (37) and (38) from $t = 1$ to $T$,

$$F(\mathbf{X}_1) - F(\mathbf{X}_{T+1}) \geq \sum_{t\in\Omega_T^1} \frac{\delta}{2}\|\mathbf{X}_{t+1} - \mathbf{Y}_t\|_F^2 + \sum_{t\in\Omega_T^2} c_1\|\mathbf{X}_{t+1} - \mathbf{X}_t\|_F^2. \quad (39)$$

As $F$ is bounded from below (Assumption A2),

$$\sum_{t\in\Omega_\infty^1} \frac{\delta}{2}\|\mathbf{X}_{t+1} - \mathbf{Y}_t\|_F^2 + \sum_{t\in\Omega_\infty^2} c_1\|\mathbf{X}_{t+1} - \mathbf{X}_t\|_F^2 \leq a_1. \quad (40)$$

where $a_1 = F(\mathbf{X}_1) - \inf F > 0$ is a constant. Consider the three cases:

1) $|\Omega_\infty^1|$ is finite but $|\Omega_\infty^2|$ is infinite: For $t_j \in \Omega_\infty^2$, we have from (40)

$$\sum_{t_j\in\Omega_\infty^2} \|\mathbf{X}_{t_j+1} - \mathbf{X}_{t_j}\|_F^2 \leq \frac{a_1}{c_1}. \quad (41)$$

From Assumption A2, we also have

$$\lim_{\|\mathbf{X}\|_F\to\infty} f(\mathbf{X}) = \infty, \quad (42)$$

which indicates that $\max_{t_j=1,\ldots,\infty}\|\mathbf{X}_{t_j}\|_F < \infty$. Together with (41), the sequence $\{\mathbf{X}_t\}$ is bounded, which has at least one limit point [47].

2) $|\Omega_\infty^1|$ is infinite but $|\Omega_\infty^2|$ is finite: For $t_j \in \Omega_\infty^1$, note that, $F(\mathbf{X}_{t_j+1}) \leq F(\mathbf{X}_{t_j})$ due to (37) and (38). From Assumption A2,

$$\inf_{\mathbf{X}} F(\mathbf{X}) > -\infty,$$

then the sequence $\{F(\mathbf{X}_{t_j})\}$ is bounded. Again, from Assumption A2, we have (42), then $\{\mathbf{X}_{t_j}\}$ is also bounded which has at least one limit point [47].

3) Both $|\Omega_\infty^1|$ and $|\Omega_\infty^2|$ are infinite: As in the above two cases, $\{\mathbf{X}_t\}$ is bounded when either of $|\Omega_\infty^1|$ and $|\Omega_\infty^2|$ is infinite.

Combining the above, $\{\mathbf{X}_t\}$ generated from Algorithm 5 is bounded and has at least one limit point. □

### A.10 Corollary 3.11

*Proof.* Let $c_2 = \min(\delta/2, c_1)$. From (39), we have

$$\begin{aligned} F(\mathbf{X}_1) - F(\mathbf{X}_{T+1}) &\geq c_2\Big(\sum_{t\in\Omega_T^1}\|\mathbf{X}_{t+1} - \mathbf{Y}_t\|_F^2 + \sum_{t\in\Omega_T^2}\|\mathbf{X}_{t+1} - \mathbf{X}_t\|_F^2\Big) \\ &= c_2\sum_{t=1}^{T}\|\mathbf{X}_{t+1} - \mathbf{C}_t\|_F^2. \end{aligned} \quad (43)$$

Thus,

$$\begin{aligned} \min_{t=1,\ldots,T}\|\mathbf{X}_{t+1} - \mathbf{C}_t\|_F^2 &\leq \frac{1}{T}\sum_{t=1}^{T}\|\mathbf{X}_{t+1} - \mathbf{C}_t\|_F^2 \\ &\leq \frac{1}{T}\sum_{t=1}^{\infty}\|\mathbf{X}_{t+1} - \mathbf{C}_t\|_F^2 \\ &\leq \frac{F(\mathbf{X}_1) - \inf F}{c_2 T}, \end{aligned}$$

where the last inequity comes from (43). □

### A.11 Theorem 3.12

*Proof.* Partition the iterations $\{1, \ldots, \infty\}$ into two sets $\Omega_\infty^1$ and $\Omega_\infty^2$, such that $t \in \Omega_\infty^1$ if step 8 is performed, and $t \in \Omega_\infty^2$ if step 10 is performed. Consider the three cases:

1) $|\Omega_\infty^1|$ is finite but $|\Omega_\infty^2|$ is infinite: Let $\{\mathbf{X}_{t_j}\}$ be a subsequence of $\{\mathbf{X}_t\}$ where $t \in \Omega_\infty^2$, and $\lim_{t_j\to\infty}\mathbf{X}_{t_j} = \mathbf{X}_*$. From (41), we have

$$\lim_{t_j\to\infty}\mathbf{X}_{t_j} = \lim_{t_j\to\infty}\mathbf{X}_{t_j+1} = \mathbf{X}_*. \quad (44)$$

Besides, using Lemma A.7, we have

$$\lim_{t_j\to\infty}\mathbf{X}_{t_j+1} = \text{InexactPS}\left(\lim_{t_j\to\infty}\mathbf{X}_{t_j}, \lim_{t_j\to\infty}\mathbf{R}_{t_j}\right). \quad (45)$$

Combining (44) and (45), we have

$$\begin{aligned} \lim_{t_j\to\infty}\mathbf{X}_{t_j+1} &= \text{InexactPS}\left(\lim_{t_j\to\infty}\mathbf{X}_{t_j}, \lim_{t_j\to\infty}\mathbf{R}_{t_j}\right) \\ &= \text{InexactPS}\left(\mathbf{X}_*, \lim_{t_j\to\infty}\mathbf{R}_{t_j}\right) = \mathbf{X}_*. \end{aligned}$$

Thus, by the assumption, we also have

$$\mathbf{X}_* = \text{prox}_{\frac{\lambda}{\tau}r}(\mathbf{X}_* - \frac{1}{\tau}\nabla f(\mathbf{X}_*)).$$

From Lemma A.8, $\mathbf{X}_*$ is also a critical point of (1).

2) $|\Omega_\infty^1|$ is infinite but $|\Omega_\infty^2|$ is finite: Let $\{\mathbf{X}_{t_j}\}$ be a subsequence of $\{\mathbf{X}_t\}$ where $t \in \Omega_\infty^1$, and $\lim_{t_j\to\infty}\mathbf{X}_{t_j} = \mathbf{X}_*$. From (39), we have

$$\sum_{t\in\Omega_\infty^1}\frac{\delta}{2}\|\mathbf{X}_{t+1} - \mathbf{Y}_t\|_F^2 < \infty$$

which indicates

$$\lim_{t_j\to\infty}\mathbf{X}_{t_j+1} - \mathbf{Y}_{t_j} = 0. \quad (46)$$

From (46), we have

$$\lim_{t_j\to\infty}\mathbf{Y}_{t_j} = \lim_{t_j\to\infty}\mathbf{X}_{t_j+1} = \mathbf{X}_*. \quad (47)$$

Besides, using Lemma A.7, we have

$$\lim_{t_j\to\infty}\mathbf{X}_{t_j+1} = \text{InexactPS}\left(\lim_{t_j\to\infty}\mathbf{Y}_{t_j}, \lim_{t_j\to\infty}\mathbf{R}_{t_j}\right). \quad (48)$$

Combining (47) and (48), we have

$$\begin{aligned} \lim_{t_j\to\infty}\mathbf{X}_{t_j+1} &= \text{InexactPS}\left(\lim_{t_j\to\infty}\mathbf{Y}_{t_j}, \lim_{t_j\to\infty}\mathbf{R}_{t_j}\right) \\ &= \text{InexactPS}\left(\mathbf{X}_*, \lim_{t_j\to\infty}\mathbf{R}_{t_j}\right) = \mathbf{X}_*. \end{aligned}$$

Thus, by the assumption, we also have

$$\mathbf{X}_* = \text{prox}_{\frac{\lambda}{\tau}r}(\mathbf{X}_* - \frac{1}{\tau}\nabla f(\mathbf{X}_*)).$$

From Lemma A.8, $\mathbf{X}_*$ is also a critical point of (1).

3) Both $|\Omega_\infty^1|$ and $|\Omega_\infty^2|$ are infinite: From the above two cases, we can see that the limit point $\mathbf{X}_*$ is also a critical point of (1) when either $|\Omega_\infty^1|$ or $|\Omega_\infty^2|$ is infinite.

Thus, limit points of $\{\mathbf{X}_t\}$ are also critical points of (1). □

## A.12 Proposition 4.1

*Proof.* Consider the two cases:

1) Steps 10 and 11 are performed: Then,

$$F(\mathbf{X}_{t+1}, \mathbf{S}_{t+1}) \leq F(\mathbf{X}_t, \mathbf{S}_t) - \frac{\delta}{2}(\|\mathbf{X}_{t+1} - \mathbf{Y}_t^{\mathbf{X}}\|_F^2 + \|\mathbf{S}_{t+1} - \mathbf{Y}_t^{\mathbf{S}}\|_F^2). \tag{49}$$

2) Steps 13 and 14 are performed: Then,

$$F(\mathbf{X}_{t+1}, \mathbf{S}_{t+1}) \leq F(\mathbf{X}_t, \mathbf{S}_t) - (c_1\|\mathbf{X}_{t+1} - \mathbf{X}_t\|_F^2 + \frac{\tau - \rho}{2}\|\mathbf{S}_{t+1} - \mathbf{S}_t\|_F^2). \tag{50}$$

Partition $\{1, \dots, T\}$ into two sets as $\Omega_T^1$ and $\Omega_T^2$, where $t \in \Omega_T^1$ if steps 10-11 are performed; otherwise, $t \in \Omega_T^2$ (and steps 13-14 are performed). Let

$$\Theta_T = \sum_{t \in \Omega_T^1} \frac{\delta}{2}(\|\mathbf{X}_{t+1} - \mathbf{Y}_t^{\mathbf{X}}\|_F^2 + \|\mathbf{S}_{t+1} - \mathbf{Y}_t^{\mathbf{S}}\|_F^2) + \sum_{t \in \Omega_T^2}(c_1\|\mathbf{X}_{t+1} - \mathbf{X}_t\|_F^2 + \frac{\tau - \rho}{2}\|\mathbf{S}_{t+1} - \mathbf{S}_t\|_F^2).$$

Summing (49) and (50) from $t = 1$ to $T$, we have

$$F(\mathbf{X}_1, \mathbf{S}_1) - F(\mathbf{X}_{T+1}, \mathbf{S}_{T+1}) \geq \Theta_T. \tag{51}$$

As $F$ is bounded from below (Assumption A2), we have

$$\Theta_\infty \leq a_2, \tag{52}$$

where $a_2 = F(\mathbf{X}_1, \mathbf{S}_1) - \inf F$. We consider the three cases:

1) $|\Omega_\infty^1|$ is finite but $|\Omega_\infty^2|$ is infinite; For $t_j \in \Omega_\infty^2$,

$$\sum_{t_j \in \Omega_\infty^2} \|\mathbf{X}_{t_j+1} - \mathbf{X}_{t_j}\|_F^2 \leq \frac{a_2}{c_1},$$
$$\sum_{t_j \in \Omega_\infty^2} \|\mathbf{S}_{t_j+1} - \mathbf{S}_{t_j}\|_F^2 \leq \frac{2a_2}{\tau - \rho}.$$

Again from Assumption A2, we have

$$\lim_{\|\mathbf{X}\|_F \to \infty \text{ or } \|\mathbf{S}\|_F \to \infty} f(\mathbf{X}, \mathbf{S}) \to \infty. \tag{53}$$

Thus, $\max_{t_j = 1, \dots, \infty} \|[\mathbf{X}_{t_j}, \mathbf{S}_{t_j}]\|_F < \infty$, and the sequence $\{[\mathbf{X}_{t_j}, \mathbf{S}_{t_j}]\}$ is bounded with at least one limit point [47].

2) $|\Omega_\infty^1|$ is infinite but $|\Omega_\infty^2|$ is finite: For $t_j \in \Omega_\infty^1$, from (49) and (50), we have $F(\mathbf{X}_{t_j+1}, \mathbf{S}_{t_j+1}) \leq F(\mathbf{X}_{t_j}, \mathbf{S}_{t_j})$. As, $F$ is bounded from below (Assumption A2), the sequence $\{F([\mathbf{X}_{t_j}, \mathbf{S}_{t_j}])\}$ must be bounded. Besides, again from Assumption A2, we have (53), which indicates the sequence $[\mathbf{X}_{t_j}, \mathbf{S}_{t_j}])$ must be bounded with at least one limit point [47].

3) Both $|\Omega_\infty^1|$ and $|\Omega_\infty^2|$ are infinite: As in the above two cases, $\{[\mathbf{X}_t, \mathbf{S}_t]\}$ is bounded with at least one limit point once $|\Omega_\infty^1|$ or $|\Omega_\infty^2|$ is infinite.

Thus, the sequence $\{[\mathbf{X}_t, \mathbf{S}_t]\}$ generated from Algorithm 5 is bounded and has at least one limit point. □

## A.13 Corollary 4.2

*Proof.* Let $c_2 = \min(\delta/2, c_1)$. First, we have

$$\sum_{t \in \Omega_T^1} \frac{\delta}{2}(\|\mathbf{X}_{t+1} - \mathbf{Y}_t^{\mathbf{X}}\|_F^2 + \|\mathbf{S}_{t+1} - \mathbf{Y}_t^{\mathbf{S}}\|_F^2) + \sum_{t \in \Omega_T^2}(c_1\|\mathbf{X}_{t+1} - \mathbf{X}_t\|_F^2 + \frac{\tau - \rho}{2}\|\mathbf{S}_{t+1} - \mathbf{S}_t\|_F^2) \geq c_2 \sum_{t=1}^{T} \|[\mathbf{X}_{t+1}, \mathbf{S}_{t+1}] - \mathbf{C}_t\|_F^2. \tag{54}$$

Together with (51) and (52), we have

$$\begin{aligned} \min_{t=1,\dots,T} &\|[\mathbf{X}_{t+1}, \mathbf{S}_{t+1}] - \mathbf{C}_t\|_F^2 \\ &\leq \frac{1}{T}\sum_{t=1}^{T} \|[\mathbf{X}_{t+1}, \mathbf{S}_{t+1}] - \mathbf{C}_t\|_F^2 \\ &\leq \sum_{t=1}^{\infty} \|[\mathbf{X}_{t+1}, \mathbf{S}_{t+1}] - \mathbf{C}_t\|_F^2 \\ &\leq \frac{F(\mathbf{X}_1, \mathbf{S}_1) - \inf F}{c_2 T}, \end{aligned}$$

where the last inequality comes from (54). □

## A.14 Theorem 4.3

*Proof.* Let $g = \breve{g} + \tilde{g}$ be the difference of convex decomposition of $g$. As two blocks of variables are involved, its critical points are defined as follows.

**Definition 3** ( [39]). *If* $\mathbf{X}$ *and* $\mathbf{S}$ *satisfy*

$$\mathbf{0} \in \nabla_{\mathbf{X}} f(\mathbf{X}, \mathbf{S}) + \lambda\left(\partial\breve{r}(\mathbf{X}) - \partial\tilde{r}(\mathbf{X})\right),$$
$$\mathbf{0} \in \nabla_{\mathbf{S}} f(\mathbf{X}, \mathbf{S}) + \lambda\left(\partial\breve{g}(\mathbf{S}) - \partial\tilde{g}(\mathbf{S})\right),$$

*then* $[\mathbf{X}, \mathbf{S}]$ *is a* critical point *of* $F$.

**Lemma A.9** ( [29]). *If* $\mathbf{X}$ *and* $\mathbf{S}$ *satisfy*

$$\mathbf{X} = \textit{prox}_{\frac{\lambda}{\tau} r}(\mathbf{X} - \frac{1}{\tau}\nabla_{\mathbf{X}} f(\mathbf{X}, \mathbf{S})),$$
$$\mathbf{S} = \textit{prox}_{\frac{\nu}{\tau} g}(\mathbf{S} - \frac{1}{\tau}\nabla_{\mathbf{S}} f(\mathbf{X}, \mathbf{S})),$$

*then* $[\mathbf{X}, \mathbf{S}]$ *is a critical point of* $F$.

Partition $\{1, \dots, \infty\}$ into two sets as $\Omega_\infty^1$ and $\Omega_\infty^2$, where $t \in \Omega_\infty^1$ if steps 10-11 are performed; otherwise, $t \in \Omega_\infty^2$ (and steps 13-14 are performed), we consider three cases here.

1) $|\Omega_\infty^1|$ is finite but $|\Omega_\infty^2|$ is infinite: Let $\{[\mathbf{X}_{t_j}, \mathbf{S}_{t_j}]\}$ be a subsequence of $\{[\mathbf{X}_t, \mathbf{S}_t]\}$ where $t \in \Omega_\infty^2$, and

$$\lim_{t_j \to \infty} [\mathbf{X}_{t_j}, \mathbf{S}_{t_j}] = [\mathbf{X}_*, \mathbf{S}_*].$$

From (51), we have

$$\sum_{t=1}^{\infty} \|\mathbf{X}_{t+1} - \mathbf{X}_t\|_F^2 < \infty, \quad \sum_{t=1}^{\infty} \|\mathbf{S}_{t+1} - \mathbf{S}_t\|_F^2 < \infty.$$

These indicate

$$\lim_{t_j \to \infty} \mathbf{X}_{t_j+1} - \mathbf{X}_{t_j} = \mathbf{0}, \tag{55}$$
$$\lim_{t_j \to \infty} \mathbf{S}_{t_j+1} - \mathbf{S}_{t_j} = \mathbf{0}. \tag{56}$$

From (55), we have

$$\lim_{t_j \to \infty} \mathbf{X}_{t_j+1} = \lim_{t_j \to \infty} \mathbf{X}_{t_j} = \mathbf{X}_*. \quad (57)$$

Combing (55) and (57), we have

$$\begin{aligned}\lim_{t_j \to \infty} \mathbf{X}_{t_j+1} &= \lim_{t_j \to \infty} \mathsf{InexactPS}\left(\mathbf{X}_{t_j}, \mathbf{R}_{t_j}\right) \quad (58)\\ &= \mathsf{InexactPS}\left(\lim_{t_j \to \infty} \mathbf{X}_{t_j}, \lim_{t_j \to \infty} \mathbf{R}_{t_j}\right)\\ &= \mathsf{InexactPS}\left(\mathbf{X}_*, \lim_{t_j \to \infty} \mathbf{R}_{t_j}\right) = \mathbf{X}_*.\end{aligned}$$

where (58) comes from Lemma A.7. Thus,

$$\mathbf{X}_* = \text{prox}_{\frac{\lambda}{\tau} r}(\mathbf{X}_* - \frac{1}{\tau}\nabla_{\mathbf{X}} f(\mathbf{X}_*, \mathbf{S}_*)) \quad (59)$$

holds by the assumption. Then, the proximal operator is always exact for $\mathbf{S}$. Using (56), we have

$$\begin{aligned}\lim_{t_j \to \infty} \mathbf{S}_{t_j+1} &= \lim_{t_j \to \infty} \text{prox}_{\frac{\mu}{\tau} g}(\mathbf{S}_{t_j} - \frac{1}{\tau}\nabla_{\mathbf{S}} f(\mathbf{X}_{t_j}, \mathbf{S}_{t_j}))\\ &= \text{prox}_{\frac{\mu}{\tau} g}(\mathbf{S}_* - \frac{1}{\tau}\nabla_{\mathbf{S}} f(\mathbf{X}_*, \mathbf{S}_*))\\ &= \mathbf{S}_* \quad (60)\end{aligned}$$

Combining with (59) and (60), $[\mathbf{X}_*, \mathbf{S}_*]$ is a critical point of (11) by using Lemma A.9.

2) $|\Omega^1_\infty|$ is infinite but $|\Omega^2_\infty|$ is finite: Let $\{[\mathbf{X}_{t_j}, \mathbf{S}_{t_j}]\}$ be a subsequence of $\{[\mathbf{X}_t, \mathbf{S}_t]\}$ where $t \in \Omega^1_\infty$, and

$$\lim_{t_j \to \infty} \left[\mathbf{X}_{t_j}, \mathbf{S}_{t_j}\right] = \left[\mathbf{X}_*, \mathbf{S}_*\right].$$

From (51), we have

$$\sum_{t_j \in \Omega^2_\infty} \|\mathbf{X}_{t_j+1} - \mathbf{Y}^{\mathbf{X}}_{t_j}\|_F^2 \leq \infty, \sum_{t_j \in \Omega^2_\infty} \|\mathbf{S}_{t_j+1} - \mathbf{Y}^{\mathbf{S}}_{t_j}\|_F^2 \leq \infty,$$

and then

$$\lim_{t_j \to \infty} \mathbf{X}_{t_j+1} - \mathbf{Y}^{\mathbf{X}}_{t_j} = \mathbf{0}, \quad (61)$$

$$\lim_{t_j \to \infty} \mathbf{S}_{t_j+1} - \mathbf{Y}^{\mathbf{S}}_{t_j} = \mathbf{0}. \quad (62)$$

Thus,

$$\lim_{t_j \to \infty} \mathbf{X}_{t_j+1} = \lim_{t_j \to \infty} \mathbf{Y}^{\mathbf{X}}_{t_j} = \mathbf{X}_*. \quad (63)$$

Combing (61) and (63), we have

$$\begin{aligned}\lim_{t_j \to \infty} \mathbf{X}_{t_j+1} &= \lim_{t_j \to \infty} \mathsf{InexactPS}\left(\mathbf{Y}^{\mathbf{X}}_{t_j}, \mathbf{R}_{t_j}\right) \quad (64)\\ &= \mathsf{InexactPS}\left(\lim_{t_j \to \infty} \mathbf{Y}^{\mathbf{X}}_{t_j}, \lim_{t_j \to \infty} \mathbf{R}_{t_j}\right)\\ &= \mathsf{InexactPS}\left(\mathbf{X}_*, \lim_{t_j \to \infty} \mathbf{R}_{t_j}\right) = \mathbf{X}_*.\end{aligned}$$

where (64) comes from Lemma A.7. Thus,

$$\mathbf{X}_* = \text{prox}_{\frac{\lambda}{\tau} r}(\mathbf{X}_* - \frac{1}{\tau}\nabla_{\mathbf{X}} f(\mathbf{X}_*, \mathbf{S}_*)) \quad (65)$$

holds by the assumption. Then, the proximal operator is always exact for $\mathbf{S}$. Using (62),

$$\begin{aligned}\lim_{t_j \to \infty} \mathbf{S}_{t_j+1} &= \lim_{t_j \to \infty} \text{prox}_{\frac{\mu}{\tau} g}(\mathbf{Y}^{\mathbf{S}}_{t_j} - \frac{1}{\tau}\nabla_{\mathbf{S}} f(\mathbf{Y}^{\mathbf{X}}_{t_j}, \mathbf{Y}^{\mathbf{S}}_{t_j}))\\ &= \text{prox}_{\frac{\mu}{\tau} g}(\mathbf{S}_* - \frac{1}{\tau}\nabla_{\mathbf{S}} f(\mathbf{X}_*, \mathbf{S}_*))\\ &= \mathbf{S}_* \quad (66)\end{aligned}$$

Combining with (65) and (66), $[\mathbf{X}_*, \mathbf{S}_*]$ is a critical point of (11) by using Lemma A.9.

3) Both $|\Omega^1_\infty|$ and $|\Omega^2_\infty|$ are infinite: As above, either $|\Omega^1_\infty|$ or $|\Omega^2_\infty|$ is infinite, a limit point $[\mathbf{X}_*, \mathbf{S}_*]$ is a critical point of (11).

Thus, the limit points of the sequence $\{[\mathbf{X}_t, \mathbf{S}_t]\}$ are also critical points of (11). □

## A.15 Proposition 5.1

*Proof.* As the SVD of $\mathbf{X}_{\text{gd}}^\top \mathbf{X}_{\text{gd}}$ is $\mathbf{V}\mathbf{\Sigma}\mathbf{V}^\top$, the SVD of $\mathbf{X}_{\text{gd}}$ can be written as $\mathbf{U}\mathbf{\Sigma}^{\frac{1}{2}}\mathbf{V}^\top$ where $\mathbf{U}$ is an orthogonal matrix containing the span of $\mathbf{X}_{\text{gd}}$. From the construction of $\mathbf{w}$, we have

$$\begin{aligned}\mathbf{X}_{\text{gd}}\mathbf{V}\left(\text{Diag}(\mathbf{w})\right)^{-\frac{1}{2}} &= \mathbf{U}\mathbf{\Sigma}^{\frac{1}{2}}(\mathbf{V}^\top\mathbf{V})\left(\text{Diag}(\mathbf{w})\right)^{-\frac{1}{2}}\\ &= \mathbf{U}\mathbf{\Sigma}^{\frac{1}{2}}\left(\text{Diag}(\mathbf{w})\right)^{-\frac{1}{2}}.\end{aligned}$$

Consider the two cases.

1) $\mathbf{X}_{\text{gd}}$ is of full column rank: Then,

$$\mathbf{U}\mathbf{\Sigma}^{\frac{1}{2}}\left(\text{Diag}(\mathbf{w})\right)^{-\frac{1}{2}} = \mathbf{U}\left(\mathbf{\Sigma}^{\frac{1}{2}}\mathbf{\Sigma}^{-\frac{1}{2}}\right) = \mathbf{U},$$

which contains the span of $\mathbf{X}_{\text{gd}}$.

2) Assume that $\mathbf{X}_{\text{gd}}$ has $k$ columns and its rank is $\bar{k} < k$: Then,

$$\begin{aligned}&\mathbf{U}\mathbf{\Sigma}^{\frac{1}{2}}\left(\text{Diag}(\mathbf{w})\right)^{-\frac{1}{2}}\\ &= \mathbf{U}\text{Diag}\left(\Sigma_{11}^{\frac{1}{2}}, \dots, \Sigma_{\bar{k}\bar{k}}^{\frac{1}{2}}, 0, \dots, 0\right)\\ &\quad \text{Diag}\left(\Sigma_{11}^{-\frac{1}{2}}, \dots, \Sigma_{\bar{k}\bar{k}}^{-\frac{1}{2}}, 1, \dots, 1\right) = \left[\mathbf{U}_{\bar{k}}, \mathbf{0}\right],\end{aligned}$$

where $\mathbf{U}_{\bar{k}}$ contains the first $\bar{k}$ columns of $\mathbf{U}$. As $\mathbf{X}_{\text{gd}}$ is only of rank $\bar{k}$, $\mathbf{U}\mathbf{\Sigma}^{\frac{1}{2}}\left(\text{Diag}(\mathbf{w})\right)^{-\frac{1}{2}}$ again covers the span of $\mathbf{X}_{\text{gd}}$.

The Proposition then follows. □

## A.16 Proposition 5.2

*Proof.* Let the SVD of $\mathbf{B}$ be $\bar{\mathbf{U}}\bar{\mathbf{\Sigma}}\bar{\mathbf{V}}^\top$. Then,

$$\mathbf{P}^\top\mathbf{B} = (\mathbf{P}^\top\bar{\mathbf{U}})\bar{\mathbf{\Sigma}}\bar{\mathbf{V}}^\top.$$

Note that

$$\begin{aligned}(\mathbf{P}^\top\bar{\mathbf{U}})^\top\mathbf{P}^\top\bar{\mathbf{U}} &= \bar{\mathbf{U}}^\top(\mathbf{P}\mathbf{P}^\top)\bar{\mathbf{U}}\\ &= \bar{\mathbf{U}}^\top(\bar{\mathbf{U}}\bar{\mathbf{U}}^\top)\bar{\mathbf{U}} = \mathbf{I},\end{aligned}$$

where the second equality comes from

$$\text{span}(\mathbf{P}) = \text{span}(\bar{\mathbf{U}}). \quad (67)$$

Thus, the SVD of $\mathbf{P}^\top\mathbf{B}$ is $(\mathbf{P}^\top\bar{\mathbf{U}})\bar{\mathbf{\Sigma}}\bar{\mathbf{V}}$. As a result, we have $\mathbf{V} = \bar{\mathbf{V}}$, $\mathbf{\Sigma} = \bar{\mathbf{\Sigma}}$. Finally, from $\mathbf{U} = \mathbf{P}^\top\bar{\mathbf{U}}$, we have

$$\mathbf{P}\mathbf{U} = \mathbf{P}\mathbf{P}^\top\bar{\mathbf{U}} = \bar{\mathbf{U}}(\bar{\mathbf{U}}^\top\bar{\mathbf{U}}) = \bar{\mathbf{U}},$$

where the second equality again comes from (67). □

## Appendix B
## The Checking Condition in [29]

In [29], an approximate $\tilde{\mathbf{X}}_p$ is accepted if $\exists \mathbf{X}_{\text{gd}} \in \partial \check{r}(\tilde{\mathbf{X}}_p) - \partial \tilde{r}(\tilde{\mathbf{X}}_p)$, where $\tilde{r}$ and $\check{r}$ are convex functions such that $\|\mathbf{X}_{\text{gd}} + \nabla f(\tilde{\mathbf{X}}_p)\|_F^2 \leq b\|\tilde{\mathbf{X}}_p - \mathbf{X}\|_F^2$ for some constant $b > 0$. Thus, to find such $\mathbf{X}_{\text{gd}}$, we first need to compute $\partial \check{r}(\tilde{\mathbf{X}}_p)$ and $\partial \tilde{r}(\tilde{\mathbf{X}}_p)$.

Taking the LSP regularizer as an example. Using Proposition 3.6, we can decompose $r(\tilde{\mathbf{X}}_p)$ as $\check{r}(\tilde{\mathbf{X}}_p)+\tilde{r}(\tilde{\mathbf{X}}_p)$, where

$$\begin{aligned}\check{r}(\tilde{\mathbf{X}}_p) &= \frac{1}{\theta}\|\tilde{\mathbf{X}}_p\|_*, \\ \tilde{r}(\tilde{\mathbf{X}}_p) &= \sum_{i=1}^{n}\left[\frac{\sigma_i(\tilde{\mathbf{X}}_p)}{\theta} - \log\left(1 + \frac{\sigma_i(\tilde{\mathbf{X}}_p)}{\theta}\right)\right].\end{aligned}$$

Let the SVD of $\tilde{\mathbf{X}}_p$ be $\mathbf{U}\mathbf{\Sigma}\mathbf{V}^\top$. Assume that $\tilde{\mathbf{X}}_p$ has $k$ singular values larger than 0. Let $\mathbf{U}_k$ (resp. $\mathbf{V}_k$) be the matrix containing the first $k$ columns of $\mathbf{U}$ (resp. $\mathbf{V}$). Then,

$$\partial \check{r}(\tilde{\mathbf{X}}_p) = \frac{1}{\theta}\left(\mathbf{U}_k\mathbf{V}_k^\top + \mathbf{B}\right),$$

where $\mathbf{B} \in \{\mathbf{C} : \mathbf{U}_k^\top \mathbf{C} = 0, \mathbf{C}\mathbf{V}_k = 0, \text{ and } \sigma_1(\mathbf{C}) \leq 1\}$. Let $\mathbf{c} = [c_i]$ with $c_i = \frac{1}{\theta} - \frac{1}{\sigma_i(\mathbf{X}_p)+\theta}$. Then,

$$\partial \tilde{r}(\tilde{\mathbf{X}}_p) = \mathbf{U}\text{Diag}(\mathbf{c})\mathbf{V}^\top.$$

Thus, a full SVD on $\tilde{\mathbf{X}}_p$ is needed, which is expensive and impractical for large matrices.

## Appendix C
## Parallel FaNCL-acc

Algorithm 11 shows the parallel version of FaNCL-acc. Acceleration is performed at step 6. The first inexact proximal step is performed at steps 8-18. Step 19 checks whether the accelerated iterate is accepted. If the condition fails, a second inexact proximal step is performed at steps 22-32. Note that the algorithm is equivalent to Algorithm 5, and thus the convergence analysis in Section 3.6 still holds.

**Algorithm 11** FaNCL-acc in parallel: FaNCL-acc-PL.

**Input:** choose $\tau > \rho$, $\lambda_0 > \lambda$, $\delta > 0$ and $\nu \in (0, 1)$;
1: initialize $\mathbf{V}_0, \mathbf{V}_1 \in \mathbb{R}^n$ as random Gaussian matrices, $\mathbf{X}_0 = \mathbf{X}_1 = 0$ and $\alpha_0 = \alpha_1 = 1$;
2: partition $\mathbf{X}_0$, $\mathbf{X}_1$, $\mathcal{P}_{\mathbf{\Omega}}(\mathbf{X}_0)$, $\mathcal{P}_{\mathbf{\Omega}}(\mathbf{X}_1)$ and $\mathcal{P}_{\mathbf{\Omega}}(\mathbf{O})$;
3: start $q$ threads for parallelization;
4: **for** $t = 1, 2, \dots T$ **do**
5: $\lambda_t = (\lambda_{t-1} - \lambda)\nu^t + \lambda$;
6: $\triangleright$ $\mathbf{Y}_t = \mathbf{X}_t + \frac{\alpha_{t-1}-1}{\alpha_t}(\mathbf{X}_t - \mathbf{X}_{t-1})$;
7: $\triangleright$ $\mathbf{R}_t =$ IndeSpan-PL $([\mathbf{V}_t, \mathbf{V}_{t-1}])$;
8: $\triangleright$ $(\mathbf{X}_{\text{gd}})_t^a = \mathbf{Y}_t - \frac{1}{\tau}\mathcal{P}_{\mathbf{\Omega}}(\mathbf{Y}_t - \mathbf{O})$;
9: **for** $p = 1, 2, \dots$ **do**
10: $\triangleright$ $[\tilde{\mathbf{X}}_p, \mathbf{R}_t] =$ ApproxGSVT-PL$((\mathbf{X}_{\text{gd}})_t^a, \mathbf{R}_t, \frac{\lambda}{\tau})$;
11: $\triangleright$ $a_p = F(\tilde{\mathbf{X}}_p)$;
12: $\triangleright$ $a_t = F(\mathbf{X}_t)$;
13: $\triangleright$ $a_F = \|\tilde{\mathbf{X}}_p - \mathbf{X}_t\|_F^2$;
14: **if** $a_p \leq a_t - c_1 a_F$ **then**
15: break;
16: **end if**
17: **end for**
18: $\triangleright$ $\mathbf{X}_{t+1}^a = \tilde{\mathbf{X}}_p$;
19: **if** $F(\mathbf{X}_{t+1}^a) \leq F(\mathbf{X}_t) - \frac{\delta}{2}\|\mathbf{X}_{t+1}^a - \mathbf{Y}_t\|_F^2$ **then**
20: $\triangleright$ $\mathbf{X}_{t+1} = \mathbf{X}_{t+1}^a$;
21: **else**
22: $\triangleright$ $(\mathbf{X}_{\text{gd}})_t = \mathbf{X}_t - \frac{1}{\tau}\mathcal{P}_{\mathbf{\Omega}}(\mathbf{X}_t - \mathbf{O})$;
23: **for** $p = 1, 2, \dots$ **do**
24: $\triangleright$ $[\tilde{\mathbf{X}}_p, \mathbf{R}_t] =$ ApproxGSVT-PL$((\mathbf{X}_{\text{gd}})_t, \mathbf{R}_t, \frac{\lambda}{\tau})$;
25: $\triangleright$ $b_p = F(\tilde{\mathbf{X}}_p)$;
26: $\triangleright$ $b_t = F(\mathbf{X}_t)$;
27: $\triangleright$ $b_F = \|\tilde{\mathbf{X}}_p - \mathbf{X}_t\|_F^2$;
28: **if** $b_p \leq b_t - c_1 b_F$ **then**
29: break;
30: **end if**
31: **end for**
32: $\triangleright$ $\mathbf{X}_{t+1} = \tilde{\mathbf{X}}_p$;
33: **end if**
34: $\alpha_{t+1} = \frac{1}{2}(\sqrt{4\alpha_t^2 + 1} + 1)$;
35: **end for**
36: **return** $\mathbf{X}_{T+1}$.
